# Supplementary material for: Subject-driven Text-to-Image Generation via Apprenticeship Learning
Source: arXiv:2304.00186 source file (2023-10-02)
Supplement: Supplementary file 1 [file z_appendix.tex]

\input{tables_and_figures/figure_results_full1}
\input{tables_and_figures/figure_results_full2}
\input{tables_and_figures/figure_results_full3}

\input{tables_and_figures/figure_kshot_full}
